# Supplementary material for: Oxygen passivation mediated tunability of trion and excitons in MoS$_2$
Source: arXiv:1707.06348 source file (2017-07-20)
Supplement: Supplementary file 1 [file Gogoi_MoS2_oxygen_SM.pdf]

# Supplemental Material

# Oxygen passivation mediated tunability of trion and excitons in $MoS_2$

Pranjal Kumar Gogoi,[1,2,*] Zhenliang Hu,[1] Qixing Wang,[1] Alexandra Carvalho,[3] Daniel Schmidt,[2] Xinmao Yin,[1] Yung-Huang Chang,[4] Lain-Jong Li,[5] Chorng Haur Sow,[1,3] A. H. Castro Neto,[1,3] Mark B. H. Breese,[1,2] Andrivo Rusydi,[1,2,6,†] and Andrew T. S. Wee[1,3,‡]

[1] *Department of Physics, Faculty of Science, National University of Singapore, Singapore 117542*
[2] *Singapore Synchrotron Light Source, National University of Singapore, 5 Research Link, Singapore 117603*
[3] *Centre for Advanced 2D Materials and Graphene Research Centre, National University of Singapore, Singapore 117542*
[4] *Department of Electrophysics, National Chiao Tung University, Hsinchu 30010, Taiwan*
[5] *Physical Science and Engineering Division, King Abdullah University of Science and Technology (KAUST), Thuwal, Saudi Arabia 23955*
[6] *NUSNNI-NanoCore, National University of Singapore, Singapore 117576*

(Dated: July 19, 2017)

## SAMPLE DETAILS

Large-area monolayer $MoS_2$ films were synthesized on sapphire(C-001 plane) substrates in a hot-wall furnace by the chemical vapour deposition method. Prior to the growth, the sapphire substrates were cleaned with standard piranha solutions. High purity $MoO_3$ (99%, Aldrich) and sulphur powder (99.5%, Alfa) were placed in two separate $Al_2O_3$ crucibles, and the substrates were placed face down on the upper side of the $MoO_3$ powder containing crucible. The $MoS_2$ samples were fabricated by annealing at 650 °C for 15 minutes with a heating rate of 15 °C per minute and under a nitrogen gas flow (1 sccm) at ambient.

Optical micrographs taken on the sample as shown in Fig. 1(a) indicate that the sample growth is uniform with almost full coverage. Photoluminescence spectra (Fig. 1(b)) taken with a laser excitation of 532 nm (WITec) show strong photoluminescence around 660 nm, which along with the characteristic Raman spectra (Fig. 1(c)) provide the evidence that it is a monolayer [1].

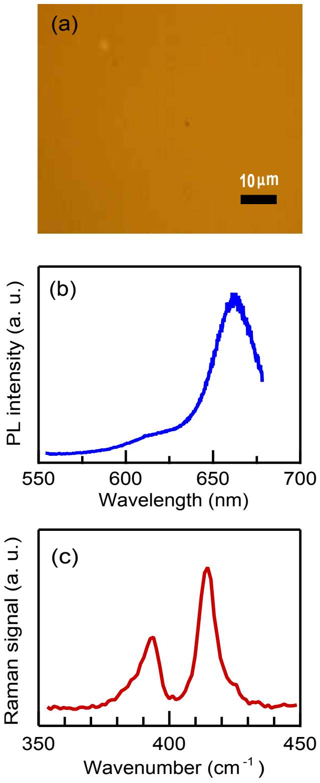


FIG. 1. Characterization of the sample. (a) Optical micrograph of $MoS_2$ monolayer sample on sapphire. (b) Photoluminescence spectra of the sample. (c) Raman spectra of the sample.

## EXPERIMENTAL DETAILS

The polarization state change of light is measured in ellipsometry either in reflection or transmission mode [2]. The measured ellipsometric angles $\Psi$ and $\Delta$ are related to the Fresnel reflection coefficients $r_p$ and $r_s$, where $p$ and $s$ represents the polarizations, by the fundamental ellipsometric equation,

$$\varrho = r_p/r_s = \tan\Psi e^{i\Delta}. \quad (1)$$

As the Fresnel reflection coefficients are related to the complex dielectric function ($\varepsilon = \varepsilon_1 + i\varepsilon_2$) of the sample, measurement of ($\Psi$, $\Delta$) allows determination of the complex dielectric function using standard modeling procedures [2]. All spectroscopic ellipsometry measurements in this work are carried out in the the reflection mode.

All the measurements in this work are performed inside the cryostat with optical windows. Since the cryostat windows are strained under UHV conditions, proper window corrections are incorporated for measurements under UHV as well as for the ones under oxygen and nitrogen

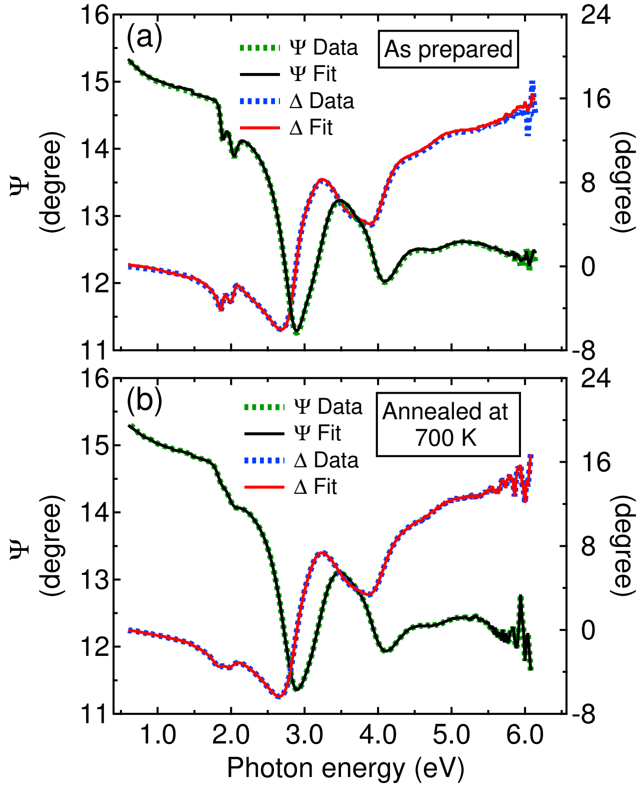


FIG. 2. Spectroscopic ellipsometry data $(\Psi, \Delta)$ and fit. (a) $(\Psi, \Delta)$ data taken on the as prepared sample at 300 K, and corresponding wavelength-by-wavelength fit result using a three layer optical model. (b) $(\Psi, \Delta)$ data taken at 300 K after annealing at 700 K in UHV, and corresponding wavelength-by-wavelength fit result using a three layer optical model. Note that for both (a) and (b) the measurements are performed in UHV.

exposure.

## COMPLEX DIELECTRIC FUNCTION $(\varepsilon_1, \varepsilon_2)$ FROM $(\Psi, \Delta)$

A wavelength-by-wavelength fit has been performed for all $(\Psi, \Delta)$ data, taken in reflection mode, using a three phase optical model ambient/$MoS_2$/sapphire. A monolayer thickness of 0.65 Å for $MoS_2$ has been used [3]. The representative experimental data $(\Psi, \Delta)$ as well as the resultant fit using the three phase model are shown in Fig. 2. In Fig. 2(a), data and fit are shown for the as prepared samples prior to any annealing (at 300 K), while Fig. 2(b) shows the data and fit for the sample after annealing at 700 K in UHV (but measured at 300 K after cooling down). The final complex dielectric function obtained from these wavelength-by-wavelength fit are shown in Fig. 1(a) and Fig. 1(b) of the main text. The complex dielectric functions for the cases of other annealing temperatures have been obtained similarly. The imaginary parts of these complex dielectric functions are used for calculating the real part of the optical conductivity as a function of energy and annealing temperature (as shown in Fig. 2(a) of the main text).

## COMPLEX DIELECTRIC FUNCTION ANALYSIS USING LORENTZIAN-GAUSSIAN OSCILLATORS

The fully Kramers-Kronig consistent Lorentzian-Gaussian osccilator is derived based on the work of Kim and Garland [4], which takes into account the analytical form of the electronic density of states. The $n^{th}$ Lorentzian-Gaussian Oscillator can be expressed as

$$\varepsilon_n(E) = iA_{\mathrm{LG}_n}\left[\int_0^\infty e^{i(E-E_n+i\gamma_n(s))s}ds - \int_0^\infty e^{i(E+E_n+i\gamma_n(s))s}ds\right] / \left[\int_0^\infty e^{-s\gamma_n(s)}ds\right] \quad (2)$$

where $\gamma_n(s) = \Gamma_n + 2{\sigma_n}^2 s$. Here $\gamma_n$ is the total broadening, and $s = t/\hbar$, $t$ is time; $\hbar$ is reduced Planck's constant; $E$ is energy; $A_{\mathrm{LG}_n}$ is a dimensionless constant. The parameters $\Gamma_n$ and $\sigma_n$ are related to the individual broadening of the Lorentzian ($B_{\mathrm{Lorentz}_n}$) and Gaussian ($B_{\mathrm{Gaussian}_n}$) components, respectively by

$$\Gamma_n = \frac{1}{2}B_{\mathrm{Lorentz}_n} \quad (3)$$

$$\sigma_n = \frac{1}{4\sqrt{\ln(4)}}B_{\mathrm{Gaussian}_n} \quad (4)$$

The complex dielectric function extracted using the wavelength-by-wavelength fit of $(\Psi, \Delta)$ for the energy range of 1.7-2.2 eV is used for these analysis. The fit details are shown in Fig. 3 for all the annealing temperatures. The real and imaginary parts of the complex dielectric function are shown in the left and right column respectively. Also note that the contributions of the first four oscillators are shown in each case. The exact parameters for each oscillator in every annealing temperature can be found in Table I, II, III, IV, V, VI, VII, VIII, and IX. In all the tables, the numbers in the parentheses give the 95% confidence limit.

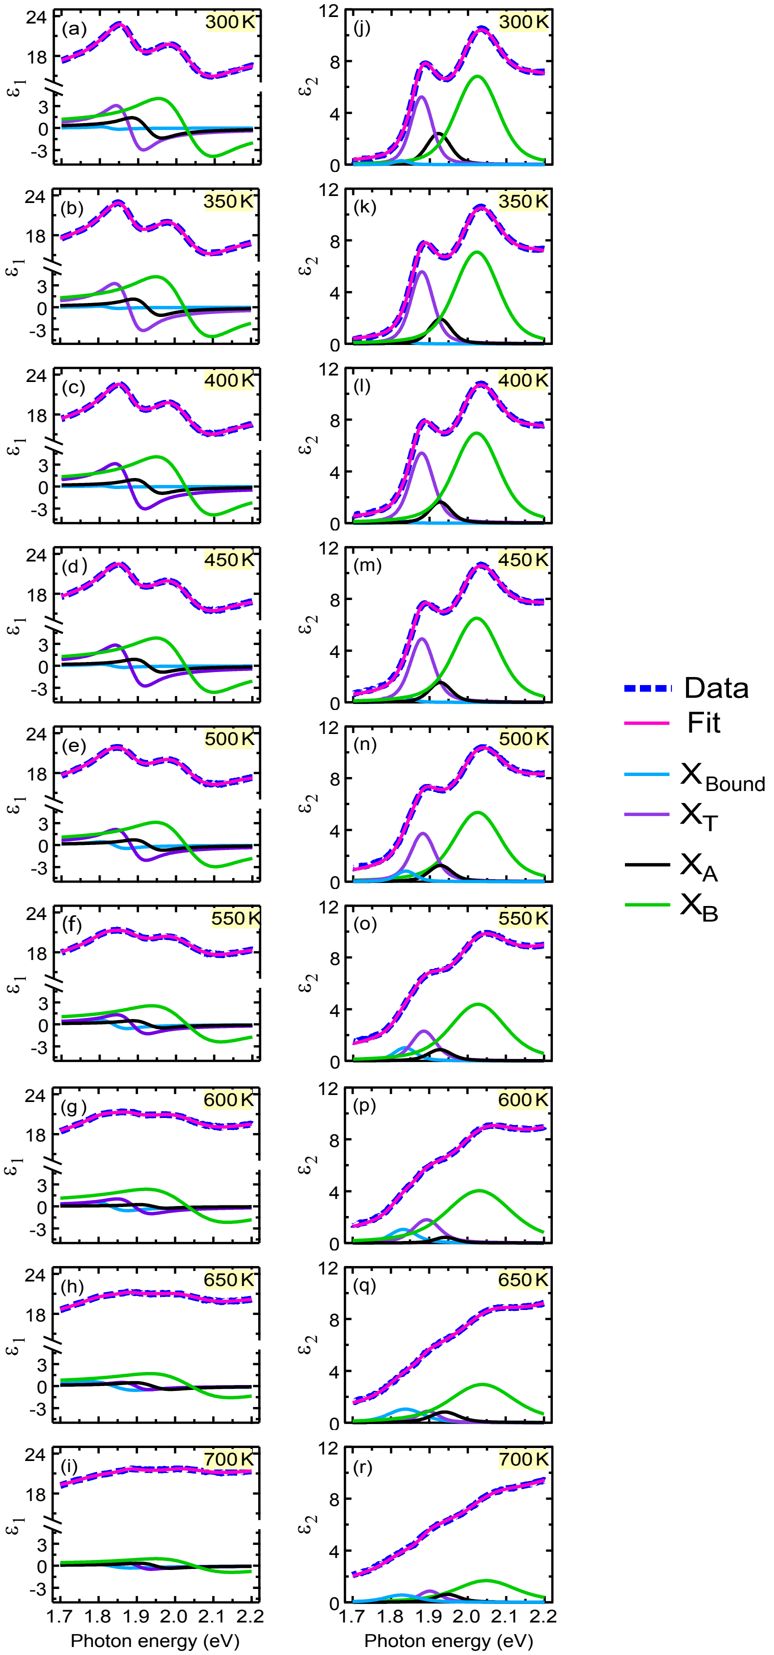


FIG. 3. Fit of the complex dielectric function ($\varepsilon_1, \varepsilon_2$) using Lorentzian-Gaussian oscillators. In (a), and (j) the fit results are shown along with the (first four) oscillators for $\varepsilon_1$, and $\varepsilon_2$ respectively for the 300 K case. The first oscillator (in cyan) corresponds to the bound exciton. The second oscillator (in purple) corresponds to the trion. The thrid (in black) and fourth (in green) oscillator corresponds to the A exciton and B exciton respectively. Similarly, for higher annealing temperatures the complex dielectric function fits are shown in the rest of the figures. The corresponding parameters for the oscillators are given in Table I, II, III, IV, V, VI, VII, VIII, and IX.

TABLE I. 300 K, $\varepsilon_1$ offset = 8.787(88), pole position = 2.471(6) eV, pole magnitude = 13.294(353).

| No. | Parameters | | |
|---|---|---|---|
| | $E_n$ (eV) | $A_{LG}$ | $\gamma$ (eV) |
| 1 | 1.826(4) | 0.30(7) | 0.039(5) |
| 2 | 1.878(2) | 5.23(50) | 0.058(1) |
| 3 | 1.923(5) | 2.40(34) | 0.064(7) |
| 4 | 2.024(3) | 6.83(6) | 0.115(1) |
| 5 | 2.191(2) | 6.70(1) | 0.287(2) |

TABLE II. 350 K, $\varepsilon_1$ offset = 8.763(92), pole position = 2.472(6) eV, pole magnitude = 13.754(360).

| No. | Parameters | | |
|---|---|---|---|
| | $E_n$ (eV) | $A_{LG}$ | $\gamma$ (eV) |
| 1 | 1.827(4) | 0.27(6) | 0.040(5) |
| 2 | 1.880(1) | 5.57(19) | 0.061(1) |
| 3 | 1.928(2) | 1.92(16) | 0.059(4) |
| 4 | 2.024(0) | 7.10(13) | 0.118(1) |
| 5 | 2.195(2) | 6.79(2) | 0.277(8) |

TABLE III. 400 K, $\varepsilon_1$ offset = 7.936(111), pole position = 2.501(8) eV, pole magnitude = 15.721(478).

| No. | Parameters | | |
|---|---|---|---|
| | $E_n$ (eV) | $A_{LG}$ | $\gamma$ (eV) |
| 1 | 1.824(6) | 0.18(10) | 0.035(8) |
| 2 | 1.880(2) | 5.48(31) | 0.063(3) |
| 3 | 1.928(5) | 1.63(32) | 0.058(6) |
| 4 | 2.023(0) | 6.96(11) | 0.121(1) |
| 5 | 2.200(2) | 6.99(2) | 0.298(8) |

TABLE IV. 450 K, $\varepsilon_1$ offset = 7.778(109), pole position = 2.528(7) eV, pole magnitude = 17.211(509).

| No. | Parameters | | |
|---|---|---|---|
| | $E_n$ (eV) | $A_{LG}$ | $\gamma$ (eV) |
| 1 | 1.834(8) | 0.38(17) | 0.048(6) |
| 2 | 1.880(3) | 4.91(24) | 0.063(0) |
| 3 | 1.928(5) | 1.54(28) | 0.060(7) |
| 4 | 2.024(4) | 6.51(6) | 0.122(1) |
| 5 | 2.208(2) | 7.21(2) | 0.325(4) |

TABLE V. 500 K, $\varepsilon_1$ offset = 6.230(144), pole position = 2.602(9) eV, pole magnitude = 23.744(793).

| No. | Parameters | | |
|---|---|---|---|
| | $E_n$ (eV) | $A_{LG}$ | $\gamma$ (eV) |
| 1 | 1.838(7) | 0.86(38) | 0.052(4) |
| 2 | 1.882(4) | 3.73(47) | 0.065(5) |
| 3 | 1.928(8) | 1.25(42) | 0.062(11) |
| 4 | 2.025(5) | 5.35(7) | 0.127(2) |
| 5 | 2.221(3) | 7.90(2) | 0.390(1) |

TABLE VI. 550 K, $\varepsilon_1$ offset = 4.298(276), pole position = 2.743(21) eV, pole magnitude = 36.02(1.99).

| No. | Parameters | | |
|---|---|---|---|
| | $E_n$ (eV) | $A_{LG}$ | $\gamma$ (eV) |
| 1 | 1.836(3) | 1.02(12) | 0.058(3) |
| 2 | 1.885(4) | 2.30(20) | 0.066(1) |
| 3 | 1.927(6) | 0.87(22) | 0.064(7) |
| 4 | 2.027(6) | 4.38(08) | 0.147(2) |
| 5 | 2.279(8) | 8.89(8) | 0.490(5) |

TABLE VII. 600 K, $\varepsilon_1$ offset = 4.562(311), pole position = 2.788(26) eV, pole magnitude = 39.538(2.41).

| No. | Parameters | | |
|---|---|---|---|
| | $E_n$ (eV) | $A_{LG}$ | $\gamma$ (eV) |
| 1 | 1.832(2) | 1.05(6) | 0.070(3) |
| 2 | 1.893(3) | 1.80(8) | 0.073(1) |
| 3 | 1.942(6) | 0.44(13) | 0.058(11) |
| 4 | 2.031(1) | 4.03(11) | 0.174(4) |
| 5 | 2.311(10) | 9.14(13) | 0.481(6) |

TABLE VIII. 650 K, $\varepsilon_1$ offset = 5.076(291), pole position = 2.748(23) eV, pole magnitude = 35.500(2.07).

| No. | Parameters | | |
|---|---|---|---|
| | $E_n$ (eV) | $A_{LG}$ | $\gamma$ (eV) |
| 1 | 1.838(5) | 1.05(10) | 0.094(6) |
| 2 | 1.897(3) | 0.89(27) | 0.059(6) |
| 3 | 1.941(7) | 0.83(16) | 0.077(11) |
| 4 | 2.039(1) | 2.95(8) | 0.173(2) |
| 5 | 2.315(10) | 9.53(13) | 0.525(8) |

TABLE IX. 700 K, $\varepsilon_1$ offset = 5.148(314), pole position = 2.772(26) eV, pole magnitude = 38.154(2.26).

| No. | Parameters | | |
|---|---|---|---|
| | $E_n$ (eV) | $A_{LG}$ | $\gamma$ (eV) |
| 1 | 1.828(2) | 0.57(4) | 0.093(5) |
| 2 | 1.901(4) | 0.87(17) | 0.060(1) |
| 3 | 1.947(7) | 0.62(15) | 0.067(16) |
| 4 | 2.048(2) | 1.68(17) | 0.163(12) |
| 5 | 2.327(21) | 9.99(20) | 0.621(14) |

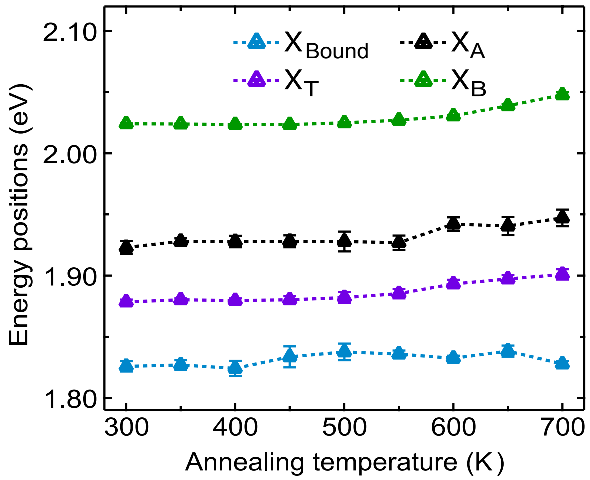


FIG. 4. Energy positions of the excitons and trion plotted against annealing temperature

## ENERGY POSITIONS OF THE OSCILLATORS

The evolution of the peak positions for $X_{\mathrm{Bound}}$, $X_{\mathrm{T}}$, $X_{\mathrm{A}}$, and $X_{\mathrm{B}}$ are shown in Fig. 4. There is an overall blueshift of the energy positions of $X_{\mathrm{T}}$, $X_{\mathrm{A}}$, and $X_{\mathrm{B}}$ with the increase of annealing temperature. However, there is an anomalous redshift of $X_{\mathrm{Bound}}$.

## DENSITY FUNCTIONAL THEORY BASED CALCULATION DETAILS, AND RESULTS

The calculations were performed using the Quantum Espresso code [5]. Geometry optimizations and total energy calculations are non-relativistic. The exchange correlation energy was described by the generalized gradient approximation (GGA), in the scheme proposed by Perdew-Burke-Ernzerhof (PBE) [6]. The energy cutoff used was 50.0 Ry. The defects were modeled in 44 $MoS_2$ supercells, where the layers were separated by a vacuum spacing of 20.7 angstroms. The energy barriers were calculated using the climbing-image nudged elastic band method [7] in the spin-average approximation.

TABLE X. Energies of the defects shown in Fig. 5

| Configuration | Relative energy (eV) |
|---|---|
| Physisorbed | 0.00 |
| B-v | -1.98 |
| B-h1 | -1.22 |
| B-h2 | -1.73 |
| D | -4.52 |

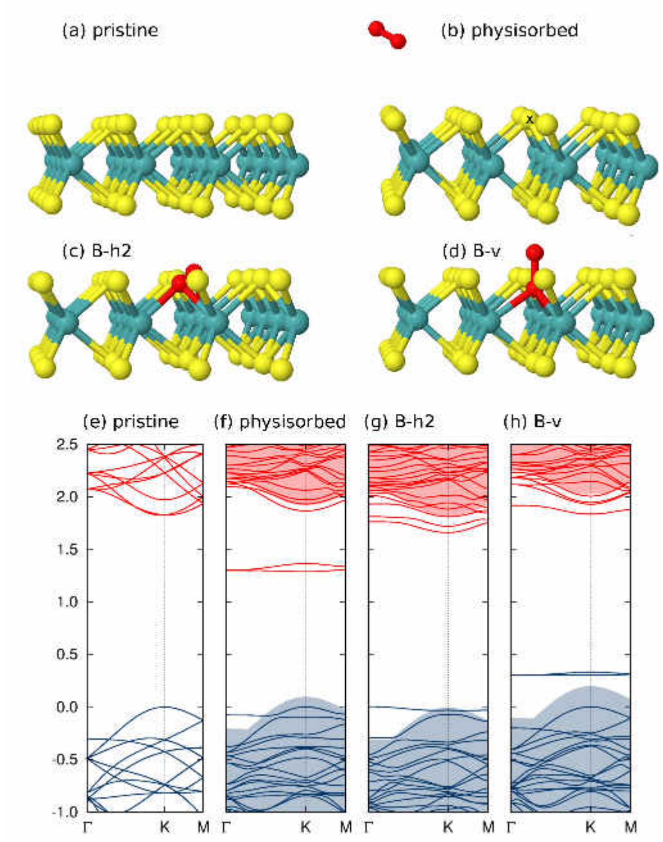


FIG. 5. Structures and respective bandstructures of (a) pristine $MoS_2$; (b) $MoS_2$ with isolated sulphur vacancy (indicated by an X); (c) oxygen chemisorbed near sulphur vacancy (spin-averaged bandstructure) in the metastable 'horizontal' configuration, and (d) oxygen molecule chemisorbed near sulphur vacancy (spin-averaged bandstructure) in the most stable 'vertical' configuration. (e-h) are the respective bandstructures. Sulphur, molybdenum and oxygen are represented by yellow, blue and red spheres, respectively. In the bandstructures, occupied levels are shown in blue,while unoccupied bands are shown in red.

.

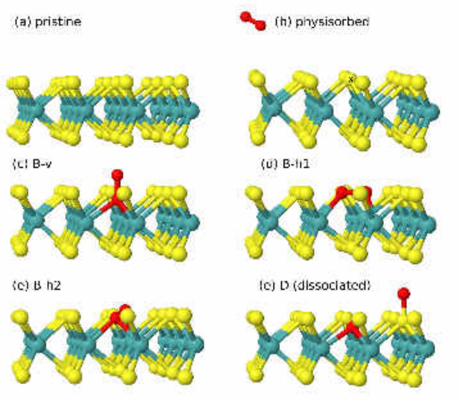


FIG. 6. Configurations of sulphur vacancy-dioxygen defects. Sulphur, molybdenum and oxygen are represented by yellow, blue and red spheres, respectively.

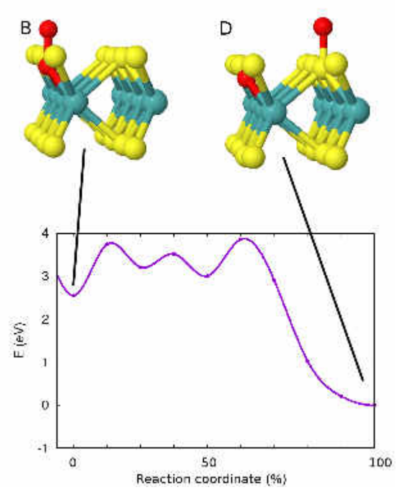


FIG. 7. Nudged elastic band calculation of the energy barrier for dissociation of the O-O bond in the sulphur vacancy-dioxygen defect shown in Fig. 6(c). The images are intermediate points along the reaction coordinate used in the nudged elastic band calculation. Top: structures before and after dissociation; Bottom: potential energy along the minimum energy path for the transformation. The calculation was performed in the spin-averaged state. A dissociation of the oxygen molecule leaving an oxygen atom at the former vacancy site would remove even the filled state leaving a totally clean gap [8]. However, this process is unlikely to happen in ambient conditions, as it requires overcoming an energy barrier of 1.23 eV.

## DESORPTION OF OXYGEN AT HIGH TEMPERATURE ULTRA HIGH VACUUM ANNEALING

Let us assume we have a dissociation reaction of the type

$$\mathrm{AB} \rightarrow \mathrm{A} + \mathrm{B}$$

where the AB complex can be, for example, the oxygen molecule chemisorbed at the vacancy site. The reaction rate will depend on the concentration of AB. Assuming a first order reaction,

$$\frac{d\,[\mathrm{AB}]}{dt} = -k\,[\mathrm{AB}]\,.$$

The reaction constant is given approximately by

$$k = \nu_0 \exp\left(-E_\mathrm{K}/(k_\mathrm{B}T)\right)$$

where $\nu_0$ is the attempt frequency. We take it to be the $O_2$ vibrational frequency, $\nu_0 \sim 5 \times 10^{13}$ Hz. $E_\mathrm{K}$ is the activation energy, which we have calculated using the nudged elastic band method for two of the most relevant transformations hypothetically taking place. The solution to the rate equation is thus given by

$$[AB] = C\exp(-kt).$$

We now consider the removal of the $O_2$ chemisorbed at the sulphur vacancies, which has an activation energy of about 2 eV. The temperature at which the concentration of the original passivated defect is reduced to half can be obtained by making

$$[AB] = C/2,$$

yielding 580 K.

* phypkg@nus.edu.sg
† phyandri@nus.edu.sg
‡ phyweets@nus.edu.sg

[1] X. Zhang, X.-F. Qiao, W. Shi, J.-B. Wu, D.-S. Jiang, and P.-H. Tan, Chem. Soc. Rev. **44**, 2757 (2015).
[2] H. Fujiwara, *Spectroscopic ellipsometry: principles and applications* (Wiley, Chichester, 2007).
[3] W. Li, A. G. Birdwell, M. Amani, R. A. Burke, X. Ling, Y.-H. Lee, X. Liang, L. Peng, C. A. Richter, J. Kong, D. J. Gundlach, and N. V. Nguyen, Phys. Rev. B **90**, 195434 (2014).
[4] C. C. Kim, J. W. Garland, H. Abad, and P. M. Raccah, Phys. Rev. B **45**, 11749 (1992).
[5] P. Giannozzi, S. Baroni, N. Bonini, M. Calandra, R. Car, C. Cavazzoni, D. Ceresoli, G. L. Chiarotti, M. Cococcioni, I. Dabo, A. D. Corso, S. de Gironcoli, S. Fabris, G. Fratesi, R. Gebauer, U. Gerstmann, C. Gougoussis, A. Kokalj, M. Lazzeri, L. Martin-Samos, N. Marzari, F. Mauri, R. Mazzarello, S. Paolini, A. Pasquarello, L. Paulatto, C. Sbraccia, S. Scandolo, G. Sclauzero, A. P. Seitsonen, A. Smogunov, P. Umari, and R. M. Wentzcovitch, J. Phys.: Condens. Matter **21**, 395502 (2009).
[6] J. P. Perdew, K. Burke, and M. Ernzerhof, Phys. Rev. Lett. **77**, 3865 (1996).
[7] G. Henkelman, B. P. Uberuaga, and H. Jónsson, J. Chem. Phys. **113**, 9901 (2000).
[8] J. Lu, A. Carvalho, X. K. Chan, H. Liu, B. Liu, E. S. Tok, K. P. Loh, A. H. C. Neto, and C. H. Sow, Nano Lett. **15**, 3524 (2015).
